# Supplementary material for: Neural-Davidsonian Semantic Proto-role Labeling
Source: arXiv:1804.07976 source file (2019-08-27)
Supplement: Supplementary file 1 [file supersenses.tex]

noun.Tops, noun.act, noun.animal, noun.artifact, noun.attribute, noun.body, noun.cognition, noun.communication, noun.event, noun.feeling, noun.food, noun.group, noun.location, noun.motive, noun.object, noun.person, noun.phenomenon, noun.plant, noun.possession, noun.process, noun.quantity, noun.relation, noun.shape, noun.state, noun.substance, noun.time
